# Supplementary material for: Generalized Schr\"odinger Bridge Matching
Source: arXiv:2310.02233 source file (2024-04-18)
Supplement: Supplementary file 1 [file appendix.tex]

\section{Review of Optimal Transport \& Stochastic Optimal Control} \label{app:review}

\newpage

\section{Proofs} \label{app:proof}

\propone*
\begin{proof}
    By fixing $p_t$ in \eq{3}, the value of $\E_{p_t}[V_t(X_t)]$ no longer depends on $\ut$, making \eq{3} the same optimization problem as in the implicit matching; see \eq{4} and Sec.~\ref{sec:2}. Since \eq{4} admits an unique minimizer $\nabla s_t^\star$, we conclude the proof.
\end{proof}

\proptwo*
\begin{proof}
Let us recall the GSB problem \eq{3} in the form of FPE constraint \eq{2}:
\begin{subequations}
    \label{eq:gsbm-fpe}
    \begin{align}
        &\min_{u_t} \int_0^1\E_{p_t}\br{\frac{1}{2}\norm{u_t(X_t)}^2 + V_t(X_t)}\dt \label{eq:gsbm} \\
    \text{s.t. }  
    \fracpartial{}{t}p_t(X_t) = - \nabla& \cdot (u_t(X_t)~p_t(X_t)) + \frac{\sigma^2}{2} \Delta p_t(X_t),
    \quad p_0 = \mu, p_1 = \nu.
    \label{eq:fpe}
    \end{align}
\end{subequations}
We seek an equivalent optimization of \eq{gsbm-fpe} given some joint coupling $p_{0,1}(x_0,x_1)$.
That is, we are only allowed to optimize $u_{t}(X_t|x_0,x_1)$ or, equivalently, $p_t(X_t|x_0, x_1)$
in the factorization $p_t = \int p_t(X_t|x_0, x_1) p_{0,1}(x_0,x_1) \rd x_0 \rd x_1$.
Under mild regularity assumptions such that Leibniz rule \citesth{} applies,
we can decompose each term in \eq{gsbm-fpe} into:
\begin{align*}
    \fracpartial{}{t} p_t(X_t) 
        &= \fracpartial{}{t} \int p_t(X_t|x_0, x_1) p_{0,1}(x_0,x_1) \rd x_0 \rd x_1
        = \E_{p_{0,1}} \br{\fracpartial{}{t} p_{t|0,1}}, \\
    \nabla \cdot \pr{u_t(X_t)~p_t(X_t)}
        &= \nabla \cdot \pr{u_t(X_t)\int p_t(X_t|x_0, x_1) p_{0,1}(x_0,x_1) \rd x_0 \rd x_1} \\
        &= \nabla \cdot \pr{\int u_t(X_t) p_t(X_t|x_0, x_1) p_{0,1}(x_0,x_1) \rd x_0 \rd x_1} \\
        &= \E_{p_{0,1}} \br{\nabla \cdot \pr{ u_t~p_{t|0,1}}}, \\
    \Delta p_t(X_t)
        &= \nabla \cdot \pr{\nabla p_t(X_t)} \\
        &= \nabla \cdot \pr{\nabla \int p_t(X_t|x_0, x_1) p_{0,1}(x_0,x_1) \rd x_0 \rd x_1} \\
        &= \E_{p_{0,1}} \br{\nabla \cdot \nabla p_{t|0,1}} \\
        &= \E_{p_{0,1}} \br{\Delta p_{t|0,1}}.
\end{align*}
We conclude the proof.
\end{proof}

\quickremark{PDE interpretation of Proposition~\ref{prop:2} and \eq{6}}
The optimal control to \eq{6} is given by 
$u^\star_t(X_t|x_0,x_1) = \sigma^2 \nabla \log \Psi_t(X_t|x_1)$, 
where the time-varying potential $\Psi_t(X_t|x_1)$ solves a partial differential equation (PDE),
well-known as the Hamilton-Jacobi-Bellman PDE:
\begin{align}\label{eq:hjb}
    \fracpartial{}{t}\Psi_t(x|x_1) = -\frac{1}{2}\sigma^2 \Delta \Psi_t(x|x_1) + V_t(x) \Psi_t(x|x_1),
    \quad 
    \Psi_1(x|x_1) = \delta_{x_1}(x).
\end{align}
In general, \eq{hjb} lacks closed-form solutions, except in specific instances. 
For example, when $V$ is quadratic, the solution is provided in \eq{u-Vquad}.
Additionally, when $V$ is degenerate, \eq{hjb} simplifies to a heat kernel, 
and its solution corresponds to the drift of the Brownian bridge utilized in DSBM \citep{shi2023diffusion}.
Otherwise, one can approximate its solution with the aid of path-integral theory (see Prop.~\ref{prop:4}).

\lmthree*
\begin{proof}
    This is a direct consequence of conditioned diffusion processes with quadratic killing rates 
    \citep{mazzolo2022conditioning},
    Specifically, \citet[Equation (84)]{mazzolo2022conditioning} gives the analytic expression 
    to the optimal control of \eq{6}, when $V_t := \alpha\norm{\sigma x}^2$:
    \begin{align}\label{eq:u-Vquad}
        u_t(X_t|x_0,x_1) = 
        \frac{\bar \sigma}{\sinh(\bar \sigma_t)} x_1 - \frac{\bar \sigma}{\tanh(\bar \sigma_t)} X_t,
    \end{align}
    where $\bar\sigma := \sigma \sqrt{2\alpha}$ and $\bar\sigma_t:=\bar\sigma(1-t)$.
    As \eq{u-Vquad} is a linear SDE, its mean $\mu_t$ and variance $\Sigma_t$ obey the following ODEs
    \citep{sarkka2019applied}:
    \begin{align} \label{eq:ode-Vquad}
        \fracdiff{\mu_t}{t} =
        \frac{\bar \sigma}{\sinh(\bar \sigma_t)} x_1 - \frac{\bar \sigma}{\tanh(\bar \sigma_t)} \mu_t,\quad
        \fracdiff{\Sigma_t}{t} =
        -\frac{2\bar \sigma}{\tanh(\bar \sigma_t)} \Sigma_t + \sigma^2\mI_d.
    \end{align}
    The analytic solution to $\mu_t$ is given by 
    \begin{align}\label{eq:mut}
        \mu_t &= \frac{ x_1 \int_0^t \pr{ \frac{\bar \sigma g_\tau}{\sinh(\bar \sigma_\tau)} } \rd \tau + K }{g_t},
    \end{align}
    where $K$ depends on the initial condition, and 
    \begin{align*}
        g_t &= \exp\pr{\int_0^t \frac{\bar \sigma}{\tanh(\bar \sigma_\tau)} \rd \tau}
            \overset{(*)}{=} \exp\pr{ \br{\ln v_t}_{\sinh(\bar\sigma_t)}^{\sinh(\bar\sigma)} }
            = \frac{\sinh(\bar\sigma)}{\sinh(\bar\sigma_t)}, \\
        \int_0^t { \frac{\bar \sigma g_\tau}{\sinh(\bar \sigma_\tau)} } \rd \tau 
            &=  \int_0^t {\frac{\bar \sigma \sinh(\bar\sigma)}{\sinh^2(\bar \sigma_\tau)}} \rd \tau 
            = \sinh(\bar\sigma) \pr{ \coth(\bar\sigma_t) - \coth(\bar\sigma)},
    \end{align*}
    where $(*)$ is due to change of variable $v_\tau:= \sinh(\bar\sigma_\tau)$.
    Substituting these results back to \eq{mut}, and noticing that $K = x_0$, yields
    \begin{align*}
        \mu_t = c_t x_0 + e_t x_1, \quad \text{where } 
        c_t = \frac{\sinh(\bar \sigma_t)}{\sinh(\bar \sigma)},\quad
        e_t = \sinh(\bar \sigma_t)\pr{\coth(\bar \sigma_t) - \coth(\bar \sigma)}.
    \end{align*}
    Following similar derivation for $\Sigma_t$, one can verify that 
    \begin{align}
        \Sigma_t 
        = \frac{\sigma^2}{\bar\sigma} \sinh^2(\bar \sigma_t)\pr{\coth(\bar \sigma_t) - \coth(\bar \sigma)}\mI_d
        = \frac{\sigma^2}{\bar\sigma} \sinh(\bar \sigma_t) e_t \mI_d
    \end{align}
    which yields the expression of $\Sigma_t = \gamma_t^2\mI_D$ in Lemma~\ref{lm:3}.
    We conclude the proof.
\end{proof}

\quickremark{Limit behavor at $t=0$ and $1$}
    Notice that $\bar\sigma_0 = \bar\sigma$ and $\bar\sigma_1 = 0$ by construction.
    Hence, one can verify that $c_0 = 1$, $e_0 = 0$, and $\gamma_0 = 0$. On the other hand,
    we have $c_1 = 0$, 
    \begin{align*}
        e_1 = \sinh(0)\pr{\frac{\cosh(0)}{\sinh(0)} - \coth(\bar \sigma)} = 1,
    \end{align*}
    which implies $\gamma_1 = 0$.
    We thus conclude that Lemma~\ref{lm:3} satisfies the boundary condition in \eq{6b}.

\quickremark{\Cref{eq:u-Vquad} recovers Brownian bridge in the limit of $\alpha\rightarrow 0$}
    Notice that 
    \begin{align*}
        \lim_{\alpha\rightarrow 0} \frac{\bar \sigma}{\sinh(\bar \sigma_t)}
        = \frac{2\bar\sigma}{e^{\bar\sigma(1-t)} - e^{-\bar\sigma(1-t)}}
        \overset{(*)}&{=} \frac{2\bar\sigma}{1 + \bar\sigma(1-t)  - (1 - \bar\sigma(1-t))}
        = \frac{1}{1-t},
    \end{align*}
    where $(*)$ is due to $\exp(x) \approx 1 + x$.
    Similarly, one can verify that 
    $\lim_{\alpha\rightarrow 0} \frac{\bar \sigma}{\tanh(\bar \sigma_t)} = \frac{1}{1-t}$.
    Hence, \eq{u-Vquad} recovers the drift of Brownian bridge \citesth{}, as expected:
    \begin{align}
        \lim_{\alpha\rightarrow 0}  u_t(X_t|x_0,x_1) = \frac{x_1 - X_t}{1-t}.
    \end{align}

\propfour*
\begin{proof}
Since the boundary constraint \eq{6b} is a Dirac delta at $x_1$,
we can transform \eq{6} into:
\begin{subequations}\label{eq:soc}
    \begin{align}
    \min_{u_{t|0,1}} \int_0^1\E_{p_t(X_t | x_0, x_1)}& 
        \br{\frac{1}{2\sigma^2}\norm{u_t(X_t|x_0, x_1)}^2 + \frac{1}{\sigma^2}V_t(X_t)}\dt 
        - \log \delta_{x_1}(X_1),
        \\
    \text{s.t. } &\rd X_t = u_t(X_t|x_0, x_1)\dt + \sigma \dWt, \quad {X_0 = x_0}
    \end{align}
\end{subequations}
where the terminal cost ``$-\log \delta_{x_1}(x)$'' vanishes at $x = x_1$ but otherwise explodes.
\Cref{eq:soc} is a valid stochastic optimal control (SOC) problem, and 
its optimal solution can be obtained as a form of path integral \citep{kappen2005path}:
\begin{align}\label{eq:pi_bb}
    p^\star(\bar X|x_0, x_1) = 
    \frac{1}{Z^\prime} \exp\pr{-\int_0^1 \frac{1}{\sigma^2} V_t(X_t)~\dt} \delta_{x_1}(X_1) q(\bar X|x_0),
\end{align}
where
$q(\cdot|x_0)$ is the density of the Brownian motion conditioned on $X_0=x_0$,
the normalization constant $Z^\prime$ is such that \eq{pi_bb} remains as a proper distribution,
and we shorthand $\bar X \equiv X_{t\in[0,1]}$.
We highlight that \Cref{eq:soc,eq:pi_bb} %
are {essential transformation} that allows us to recover 
the conditional distribution used in prior works \citep{shi2023diffusion} when $V_t:=0$ (see remarks below)

Directly re-weighting samples from $q$ using \eq{pi_bb} may have poor complexity
as most samples are assigned with zero weights due to $\delta_{x_1}(\cdot)$.
An more efficient alternative is to rebase the sampling distribution in \eq{pi_bb} from $q$ to 
an importance sampling $r(\bar X|x_0, x_1)$ such that $X_0 = x_0$, $X_1 = x_1$,
and is absolutely continuous with respect to $q$.
Then, the remarkable results from information-theoretic SOC 
\citep{theodorou2010generalized,theodorou2015nonlinear} suggest
\begin{align}\label{eq:pi_gsbm}
    p^\star(\bar X|x_0, x_1) = 
    \frac{1}{Z} \exp\pr{-\int_0^1 \frac{1}{\sigma^2} V_t(X_t)~\dt} \frac{q(\bar X|x_0)}{r(\bar X|x_0, x_1)} r(\bar X|x_0, x_1)
\end{align}
where the Radon-Nikodym derivative $\frac{q}{r}$ can be computed via Girsanov's theorem \citep{sarkka2019applied}, 
given by \eq{gir-thm}. 
We conclude the proof.
\end{proof}

\quickremark{\Cref{eq:pi_bb} recovers Brownian bridge when $V_t:=0$}
    One can verify that, when $V_t:=0$, the optimal solution
    $p^\star(\bar X|x_0, x_1) \propto \delta_{x_1}(X_1) q(\bar X|x_0)$ is simply 
    the Brownian motion \emph{conditioned} on the end point being $x_1$, 
    which is precisely the definition of Brownian bridge \citesth{}.
    Notice how we also recover the result in Lemma~\ref{lm:3}.

\thmfive*
\begin{proof}
    Denote the the intermediate results of Stage 1 and 2, after repeating $n$ times, respectively
    by $p_t^n$ and $p_{t|0,1}^n$.
    Under mild assumptions \citep{anderson1982reverse,yong1999stochastic} such that all distributions approach zero at a sufficient speed as $\norm{x} \rightarrow \infty$, and that all integrands are bounded, we have (note that inputs to all functions are dropped for notational simplicity):
    \begin{align*}
        \calL(\theta^n) %
        &= \int\int p_t^n \pr{\frac{1}{2}\norm{u_t}^2 + V_t} \rd x_t \dt \\
        &= \int p_{0,1}^n {\br{\int\int q^n_{t|0,1} \pr{\frac{1}{2}\norm{u_t}^2 + V_t} \rd x_{t|0,1} \dt}} \rd x_{0,1}  && \text{\color{gray} by Fubini's Theorem} \\
        &\ge
            \int p_{0,1}^n {\br{\int\int p_{t|0,1}^{n} \pr{\frac{1}{2}\norm{u_t}^2 + V_t} \rd x_{t|0,1} \dt}} \rd x_{0,1} &&  \text{\color{gray} by optimizing \eq{6}} \\
        &= \int\int q_t^{n} \pr{\frac{1}{2}\norm{u_t}^2 + V_t} \rd x_t \dt && \text{\color{gray} by Fubini's Theorem} \\
        &\ge \int\int p_t^{n+1} \pr{\frac{1}{2}\norm{u_t}^2 + V_t} \rd x_t \dt  \numberthis \label{eq:thm6} \\
        &= \calL(\theta^{n+1}),
    \end{align*}
    where we factorize the solution of Stage 1 by
    $p^n_t := \int p^n_{0,1} q^n_{t|0,1} \rd x_{0,1}$, and marginalize
    the solution of Stage 2 by $q_t^{n} := \int p_{0,1}^n p_{t|0,1}^{n} \rd x_{0,1}$.
    The inequality in \eq{thm6} follows from the fact that $p_t^{n+1}$,  as the solution to the next Stage~1, finds the unique minimizer that yields the same marginal as $q_t^n$ while minimizing kinetic energy, \ie 
    \begin{align*}
        \int q_t^n~V_t~\rd x_t = \int p_t^{n+1}~V_t~\rd x_t, \quad 
        \int q_t^n~\norm{u_t}^2~\rd x_t \ge \int p_t^{n+1}~\norm{u_t}^2~\rd x_t.
    \end{align*}
\end{proof}
    
\thmsix*
\begin{proof}
    Let $p_t^\star$ 
    and $u_t^\star$ be the optimal solution to the GSB problem in \eq{3}, and 
    suppose $p_t^\star := \int p_{t|0,1}^\star p_{0,1}^\star \rd x_0 \rd x_1$.
    It suffices to show that 
    \begin{enumerate}
        \item Given $x_0,x_1 \sim p_{0,1}^\star$, the conditional distribution $p_{t|0,1}^\star$ is the optimal solution to \eq{6}.
        \item Given $p_t^\star$, both matching algorithms (\Algref{iml} and \ref{alg:exp}) return $u_t^\star$.
    \end{enumerate}
    The first statement follows directly from the Forward-Backward SDE (FBSDE) 
    representation of \eq{3}, initially derived in \citet{liu2022deep}.
    Specifically, the theory suggests that the (conditional) optimal control bridging
    any $x_0,x_1 \sim p_{0,1}^\star$ satisfies a BSDE \citep{pardoux2005backward} 
    that is uniquely associated with the HJB PDE of \eq{6}, \ie \eq{hjb}.
    This readily implies that $p_{t|0,1}^\star$ is the solution to \eq{6}.

    Since $u_t^\star$ is known to be a 
    gradient field \citep[Equation (3)]{liu2022deep}, it must coincide with the solution returned by the
    implicit matching algorithm (\Algref{iml}), as $\Limp$ seeks the unique gradient field that matches $p_t^\star$.
    On the other hand, since the explicit matching loss \eq{5} can be interpreted as a 
    Markovian projection \citep{shi2023diffusion}, \ie 
    it returns the closet (in the KL sense) Markovian process w.r.t. 
    the reciprocal path measure \citep{leonard2013survey,leonard2014reciprocal}
    defined by the solution to \eq{6}.
    Since the solution to \eq{6}, as proven in the first statement, is simply $p_{t|0,1}^\star$,
    the closet Markovian process is by construction $u_t^\star$.
    Hence, the second statement also holds, and we conclude the proof.\footnote{
        It is important to note that, while $\Lexp$ and $\Limp$ do not share the same minimizer in general, 
        they do at the equilibrium $p_t^\star$.
    }

\end{proof}

\section{Additional Derivations and Discussions}\label{app:other-derivation}

\subsection{Explicit matching loss}\label{app:bm}

\paragraph*{How \eq{5} preserves the prescribed $p_t$.}

The rigorous derivation of the explicit matching loss \eq{5} can be found in, \eg \citet[Proposition 2]{shi2023diffusion}, 
called \emph{Markovian projection}. Here, we provide an alternative derivation
that follows closer to the one from flow matching \citep{lipman2022flow}.
\begin{restatable}{lm}{lmseven}\label{lm:7}
    Let the marginal $p_t$ be constructed from a mixture of conditional probability paths, \ie
    $p_t := \E_{p_{0,1}}[p_t(X_t|x_0, x_1)]$, where $p_t(X_t|x_0, x_1) \equiv p_{t | 0, 1}$ 
    is associated with an SDE, $\rd X_t = u_t(X_t|x_0,x_1) \dt + \sigma \dWt$, then 
    the SDE drift that satisfies the FPE prescribed by $p_t$ is given by
    \begin{align}\label{eq:bm-u}
        u^\star_t(x) = \frac{\E_{p_{0,1}}[u_t(x|x_0,x_1)]}{p_t(x)}
    \end{align}
\end{restatable}
\begin{proof}
    It suffices to check that $u^\star_t(x)$ satisfies the FPE prescribed by $p_t$:
    \begin{align*}
        \fracpartial{}{t}p_t(X_t)
        &= \int \pr{\fracpartial{}{t} p_{t | 0, 1}} p_{0,1} \rd x_0 \rd x_1 \\
        &= 
        \int \pr{ - \nabla \cdot \pr{ u_{t | 0, 1}~p_{t | 0, 1} } } p_{0,1} \rd x_0 \rd x_1 
        + \int \pr{ \frac{1}{2}\sigma^2 \Delta p_{t | 0, 1} } p_{0,1} \rd x_0 \rd x_1 
        \\
        \overset{\text{\eq{bm-u}}}&{=} - \nabla \cdot \pr { u^\star_t~p_t } + \frac{1}{2}\sigma^2 \Delta p_t.
    \end{align*}
\end{proof}
An immediate consequence of Lemma~\ref{lm:7}, following standard treatments \citep{vincent2011connection}, is that 
\begin{align}\label{eq:bm-loss-v2}
    \Lexp(\theta)
    = \E_{p_t} \br{\frac{1}{2}\norm{u_t^\theta(X_t) - u^\star_t(X_t)}^2} + \calO(1),
\end{align}
where $\calO(1)$ is independent of $\theta$. 
Hence, the $u_t^{\theta^\star}$ preserves the prescribed $p_t$.

\paragraph*{Relation to implicit matching \eq{4}.}
As shown in Sec.~\ref{sec:2} and \eq{bm-loss-v2}, both explicit and implicit matching losses can be associated with regression objectives averaged over $p_t$, except with the different targets, \ie $u^\star_t$ and $\nabla s^\star_t$.
As pointed out in \citet{neklyudov2022action},
these targets can be related through the Helmholtz decomposition \citep[Lemma 8.4.2]{ambrosio2008gradient},
suggesting that $u^\star_t = \nabla s^\star_t + w_t$ where $w_t$ is the divergence-free vector field, \ie $\nabla\cdot(w_t p_t) = 0$.
Though this implies that $\Lexp$ only upper-bounds the kinetic energy,
its solution sequential, by alternating between solving \eq{6} in Stage 2,
remains well-defined from the measure perspective \citep{peluchetti2021non,peluchetti2023diffusion,shi2023diffusion}.
Specifically, the sequential performs alternate projection between 
reciprocal path measure defined by the solution to \eq{6}, in the form $p_t := \E_{p_{0,1}}[p_{t|0,1}]$,
and the Markovian path measure, and admit convergence to the optimal solution for standard SB problems.

\subsection{Gaussian probability path}\label{app:gpath}

\paragraph*{Derivation of analytic conditional drift in \eq{8}.}

Recall the Gaussian path approximation in \eq{7}:
\begin{align*}
    X_t = \mu_t + \gamma_t Z, \quad Z \sim \calN(0,\mI_d),
\end{align*}
which immediately implies the velocity vector field 
and the score function \citep{sarkka2019applied,albergo2023stochastic}:
\begin{align*}
    \partial_t X_t 
    = \partial_t \mu_t + \frac{\partial_t \gamma_t}{\gamma_t} \pr{X_t - \mu_t}, \quad 
    \nabla \log p_t(X_t) 
    = -\frac{1}{\gamma_t^2} \pr{X_t - \mu_t}.
\end{align*}
We can then construct the conditional drift 
following standard practices \citep{song2021maximum}:
\begin{align}\label{eq:8v2}
    u_t(X_t|x_0, x_1) 
    = \partial_t X_t + \frac{\sigma^2}{2} \nabla \log p_t(X_t)
    = \partial_t \mu_t + \frac{1}{\gamma_t}\pr{\partial_t \gamma_t - \frac{\sigma^2}{2\gamma_t}} (X_t - \mu_t).
\end{align}
Notice that \eq{8v2} is of the form of a gradient field due to the linearity in $X_t$.

One can verify that when
$\mu_t := (1-t)x_0 + t x_1$ and $\gamma_t := \sigma \sqrt{t(1-t)}$,
as the solution to Brownian bridge,
\eq{8v2} yields the desired drift of Brownian bridge $\frac{x_1 - X_t}{1-t}$.

\paragraph*{Efficient simulation with analytic covariance function (\Cref{ft:4}).} %

Proposition~\ref{prop:4} requires sampling from the ``\emph{joint}'', \ie path-wise, 
distribution. For general nonlinear SDE, this requires sequential simulation, which can scale poorly 
to higher-dimensional applications.
Fortunately, there exists efficient computation for the Gaussian paths \eq{7}.
We detail the derivation, following standard practices \citep{sarkka2019applied}, 
below for completeness.

Firstly, notice that the solution of \eq{7} and \eq{8} is
\begin{align}\label{eq:gt}
    X_t = e^{g_t} \pr{x_0 + \int_0^t e^{-g_\tau} b_t \rd \tau 
                            + \int_0^t e^{-g_\tau} \sigma \rd W_s 
                        },\quad
    g_t := \int_0^t a_\tau \rd \tau,
\end{align}
where $a_t := \frac{1}{\gamma_t}\pr{\partial_t \gamma_t - \frac{\sigma^2}{2\gamma_t}}$ is defined in \eq{8},
$b_t := \partial_t \mu_t - a_t \mu_t$ and
$\int[\dots]\rd W_s$ is the Ito stochastic integral \citesth{check nsde ref}.
The covariance function given any $0\le s < t \le 1$ can be computed by
\begin{align*}
    \Cov(s, t) &= e^{g_s + g_t}
    \langle \int_0^s e^{-g_\tau} \sigma \rd W_\tau, \int_0^t e^{-g_\tau} \sigma \rd W_\tau \rangle \\
    \overset{(i)}&{=} e^{g_s + g_t} \langle \int_0^s e^{-g_\tau} \sigma \rd W_\tau, \int_0^s e^{-g_\tau} \sigma \rd W_\tau \rangle \\
    \overset{(ii)}&{=} e^{g_s + g_t} \int_0^s e^{-2g_\tau} \sigma^2 \dt \\
    \overset{(iii)}&{=} e^{g_t - g_s}~\Var(s) \\
    \overset{\text{\eq{7}}}&{=} e^{g_t - g_s}~\gamma_s^2 \numberthis \label{eq:cov-dev}
\end{align*}
where $(i)$ is due to the independency of the Ito integral between $[0,s]$ and $[s,t]$,
$(ii)$ is due to the Ito isometry, and, finally,
$(iii)$ is due to substituting $\Var(s) := e^{2g_s} \int_0^s e^{-2g_\tau} \sigma^2 \dt$.

Repeating the same derivation for $t < s$, 
the covariance function of \eq{7} between any given two timesteps $s,t \in [0,1]$
can be written cleanly as 
\begin{align}\label{eq:cov}
    \Cov(s, t) = \gamma_{\min(s,t)}^2 e^{g_{\max(s,t)} - g_{\min(s,t)}},
\end{align}
which, crucially, requires only solving an ``1D'' ODE, $\rd g_t = a_t \dt, g_0 = 0$. 
We summarize the algorithm in Alg.~\ref{alg:covsample}. 
Notice again that all computation is parallelizable over the batches.

\begin{figure}[H]
    \centering 
    \begin{minipage}{0.38\textwidth}
        \centering
        \includegraphics[width=0.8\linewidth]{fig/cov_sample.png}
        \label{fig:cov}
        \vskip -0.1in
        \caption{
            How Alg.~\ref{alg:covsample} faithfully recovers the covariance matrix of, in this case, Brownian bridge.
        }
    \end{minipage}
    \hfill
    \begin{minipage}{0.6\textwidth}
       \begin{algorithm}[H]
          \caption{\texttt{CovSample} (line 1 in Alg.~\ref{alg:pi})}
          \label{alg:covsample}
          \begin{algorithmic}
          \Require SDE \eq{6b} with $\mu_t, \gamma_t$
          \State Discretize $\bar t := [t_1, \cdots, t_K]$,~~$0 < t_1 < \cdots < t_K < 1$
          \State Solve 1D ODE $g_{\bar t}$ according to \eq{gt}
          \State Compute covariance matrix $C_{\bar t} \in \R^{K\times K}$ by \eq{cov}
          \State Perform Cholesky decomposition $ C_{\bar t} = L_{\bar t} L_{\bar t}^T$
          \State Sample 
            $X_{\bar t} = \mu_{\bar t} + L_{\bar t} Z_{\bar t} $, 
            $Z_{\bar t} \in \R^{K\times d}$,
            $[Z_{\bar t}]_{ij} \sim \calN(0,1)$
          \State \Return $X_{\bar t}$
          \end{algorithmic}
       \end{algorithm}
    \end{minipage}
\end{figure}

\section{Experiment Details} \label{app:exp}

\subsection{Experiment setup}\label{app:setup}

\paragraph{Baselines.}
All experiments on DeepGSB are run with their official implementation\footnote{
    \url{https://github.com/ghliu/DeepGSB}, under Apache License.
} and default hyperparameters. 
Specifically, we adopt the ``actor-critic'' parameterization as it generally yields better performance.
It is however worth noting that this approach requires additional parameterization for the value networks.
On the other hand, we implement DSBM ourselves in the AFHQ task. Our GSBM can be made equivalent to DSBM by disabling the optimization of the CondSOC problem in \eq{6} and returning the analytic solution of Brownian bridges instead. This enables us to more effectively isolate and study the algorithmic differences, ensuring that any performance gaps are solely attributable to the presence of $V_t$.

\paragraph{Network architectures.}
For crowd navigation (Sec.~\ref{sec:crowd-nav}) and opinion depolarization (Sec.~\ref{sec:opinion}), we adopt the same network architectures as in DeepGSB, which consists of 4-5 residual blocks with sinusoidal time embedding.
As for the AFHQ task, we consider $\ut$ as U-Net \citep{ronneberger2015u} from the implementation of 
\citet{dhariwal2021diffusion}.\footnote{
    \url{https://github.com/openai/guided-diffusion}, under MIT License.
}
All networks are trained from scratch, without utilizing any pretrained checkpoint, and optimized with AdamW \citep{loshchilov2017decoupled}.

\paragraph{Task-specific noise level ($\sigma$).}
All tasks on crowd navigation with mean-field cost adopt $\sigma = \{1.0, 2.0\}$,
whereas the opinion depolarization task uses $\sigma=0.5$.
These values are directly adopted from DeepGSB.
On the other hand, we use $\sigma=1$ and $0.5$ respectively for Lidar and AFHQ tasks.

\paragraph{GSBM implementation (forward \& backward scheme).}
In practice, we employ similar ``forward and backward'' scheme proposed in DSBM \citep{shi2023diffusion}, parameterizating two SDE drifts, one for the forward simulation and another for the backward.
During odd epochs, we simulate the coupling (line 4 in Alg.~\ref{alg:gsbm}) from the forward drift, solve the corresponding CondSOC problem \eq{6}, then match the resulting $p_t$ with the backward drift. 
Conversely, during even epochs, we follow the reverse process, matching the forward drift with the $p_t$ obtained from backward drift.
The forward-backward alternating scheme generally improves the performance as the forward drift always matches the ground-truth terminal distribution $p_1 = \nu$ (and vise versa for the backward drift).

\paragraph{GSBM hyperparameters.}
\Cref{tb:hyperparam} summarizes the hyperparameters used in the spline optimization. By default, the generation processes are discretized into 1000 steps, except for the opinion depolarization task, where we follow DeepGSB and discretize into 300 steps.

\begin{table}[H]
    \caption{
        Hyperparameters of the \texttt{SplineOpt} (Alg.~\ref{alg:spline}) for each task.
    }
    \label{tb:hyperparam}
    \centering
    \vskip -0.07in
    \begin{tabular}{lcccccc}
        \toprule
        & Stunnel & Vneck   & GMM     & Lidar   & AFHQ    & Opinion \\
        \midrule
        $K$       & 30 & 30 & 30 & 30  & 8 & 30 \\[2pt]
        $M$       & 1000 & 3000 & 2000 & 200  & 100 & 700 \\[2pt]
        $|i|$     & 4 & 4 & 4 & 4  & 4 & 4 \\[2pt]
        Optimizer & SGD &  SGD & SGD & mSGD & Adam & SGD    \\[2pt]
        \bottomrule
    \end{tabular}
\end{table}

\begin{wrapfigure}[12]{r}{0.41\textwidth}
    \vspace*{-10pt}
    \centering
    \includegraphics[width=0.41\textwidth]{fig/crowd_nav_2d_p0_p1.png}
    \vskip -0.1in
    \caption{
        Initial ($\mu$, marked blue) and terminal ($\nu$, marked orange) distributions 
        for each crowd navigation task with mean-field state cost. 
        The obstacles are marked gray.
    }
    \label{fig:crowd_nav_2d_p0_p1}
\end{wrapfigure}
\paragraph{Crowd navigation setup.}
All three mean-field tasks---namely Stunnel, Vneck, and GMM---are directly adopted from DeepGSB,
as shown in Fig.~\ref{fig:crowd_nav_2d_p0_p1}.
We slightly modify the initial distribution of the GMM to testify multi-to-multi modal transportation.
As for the mean-field interaction cost \eq{V-mf}, we consider entropy cost for the Vneck task, and congestion cost for the Stunnel and GMM tasks.
In practice, we soften the obstacle cost for differentiability, similar to prior works \citep{ruthotto2020machine,lin2021alternating}, and approximate $p_t(x) \approx \sum_{(x_0,x_1)} p_t(x|x_0,x_1)$ as the mixture of Gaussian paths given in \eq{7}, where each $p_t(x|x_0,x_1)$ is a Gaussian whose kernel is determined via $\sigma$.

\paragraph{AFHQ setup.}

As our state cost $V_t$ is defined via a latent space, we pretrained a $\beta$-VAE \citep{higgins2016beta} with 
$\beta=0.1$. Next, we note that the spherical linear interpolation (Slerp: \citet{shoemake1985animating}) can be computed via
\begin{align}
    I_{\text{Slerp}}(t,z_0,z_1) := 
        \frac{\sin((1-t)~\Omega)}{\sin\Omega} z_0 + \frac{\sin(t~\Omega)}{\sin\Omega} z_1,\qquad
        \Omega = \arccos(\langle z_0,z_1 \rangle),
\end{align}
which refers to constant speed rotation motion along a great circle arc.
